# Supplementary material for: Exploring the free energy gain of phase separation via Markov State Modeling
Source: arXiv:1705.01409 source file (2017-06-08)
Supplement: Supplementary file 1 [file SupplementaryMaterial.pdf]

## SUPPLEMENTARY MATERIAL

### Free energy differences for various system sizes

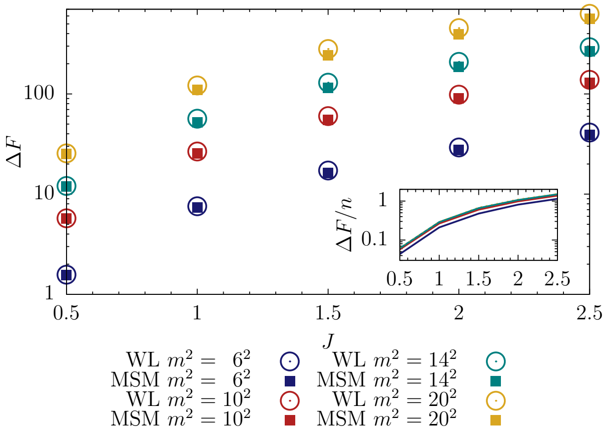


Figure 1. Free energy differences between mixed and phase-separated configurations as a function of the interaction parameter between spins for various system sizes. The inset displays the same free energy differences but normalized by the total number of spins in the system, $n = m^2$. The order parameter of average mixed configurations is given by the size of the system, $N_{\text{mixed}} = \frac{m^2}{2}$, whereas the order parameter of the phase-separated configurations depends on both the interaction parameter and the size of the system and can be determined as the order parameter with minimal free energy.

## Comparison of the finer $N + \mathrm{Var}$ discretization scheme with the absent-connections algorithm

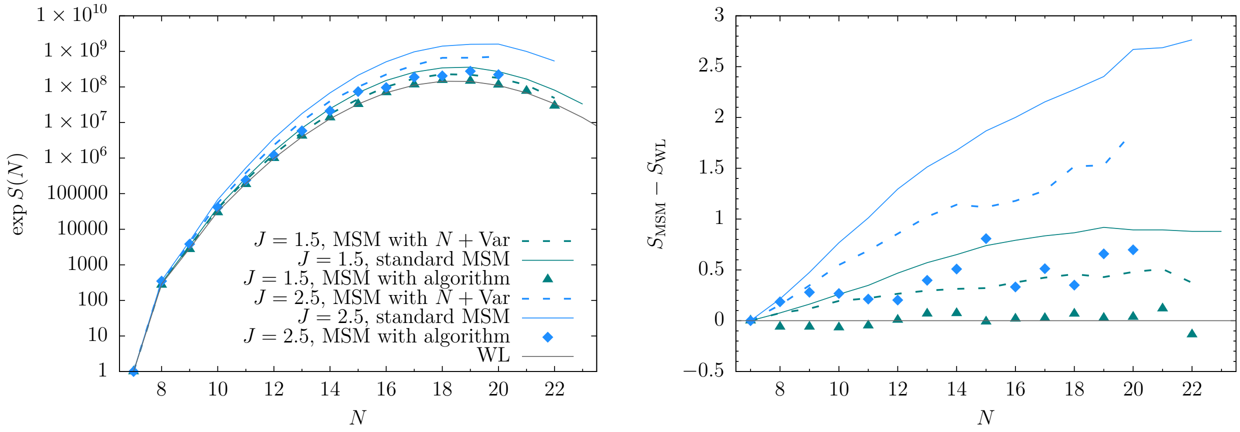


Figure 2. Density of states per order parameter and entropy differences $S_{\mathrm{MSM}} - S_{\mathrm{WL}}$ in a $6^2$ sized Ising system computed via MSM with the $N$ discretization scheme (coloured lines), MSM with the $N + \mathrm{Var}$ discretization scheme (dashed lines), MSM with $N$ discretization and application of the absent-connections algorithm (symbols) and WL sampling (grey line), respectively.

## Additional data from the analytic solution of the five state model system

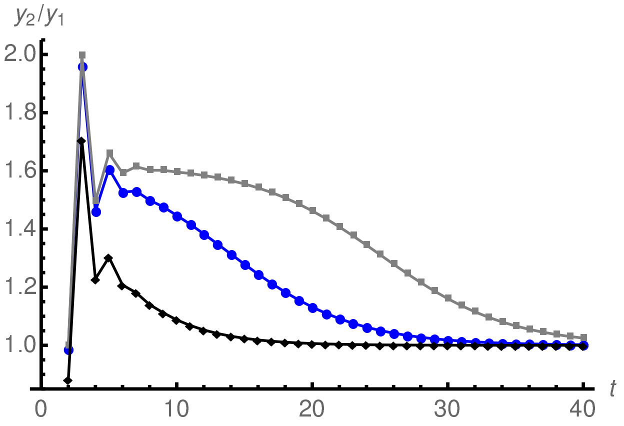


Figure 3. Evolution of the ratio $y_2(t)/y_1(t)$ for case II (initial population $\mathbf{y}^T(0) = (0, 1, 0)$) with the number of MC steps. The colour coding corresponds to different values of $\varepsilon$ according to: blue $\rightarrow \varepsilon = \exp(-5)$, grey $\rightarrow \varepsilon/10$ and black $\rightarrow \varepsilon \cdot 10$. Because the initial population of $y_2(0) = 0$, the points only start after $y_2$ has gained some population (here: after two MC steps).

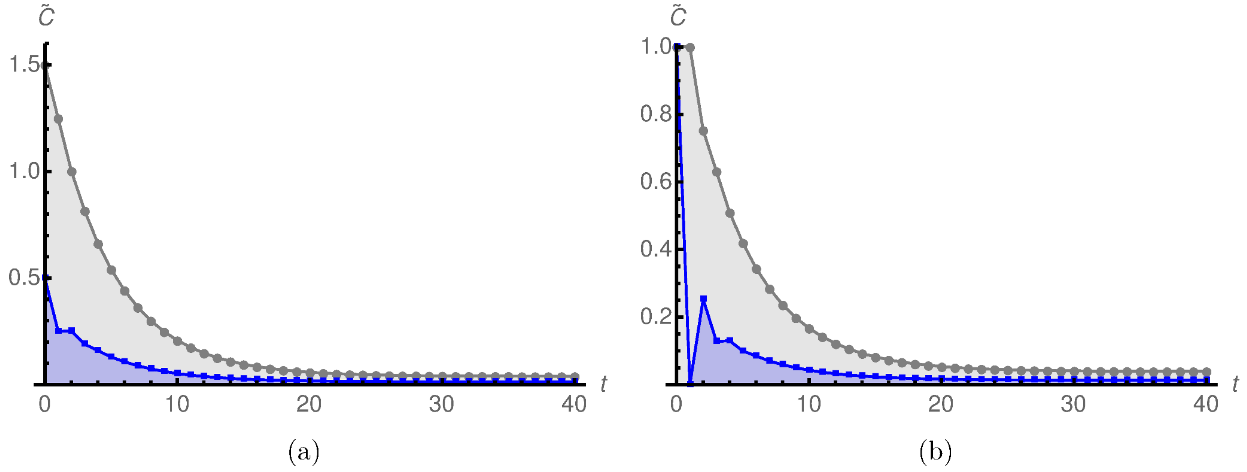


Figure 4. Numbers of transitions per MC step $\widetilde{C}_{\mathrm{BB}}$ (grey) and $\widetilde{C}_{\mathrm{BA}}$ (blue) in the five state model system. a): locally equilibrated initial distribution in Markov state B, $\mathbf{y}^T(0) = (0, \frac{1}{2}, \frac{1}{2})$; b): locally non-equilibrated initial distribution in Markov state B, $\mathbf{y}^T(0) = (0, 1, 0)$.

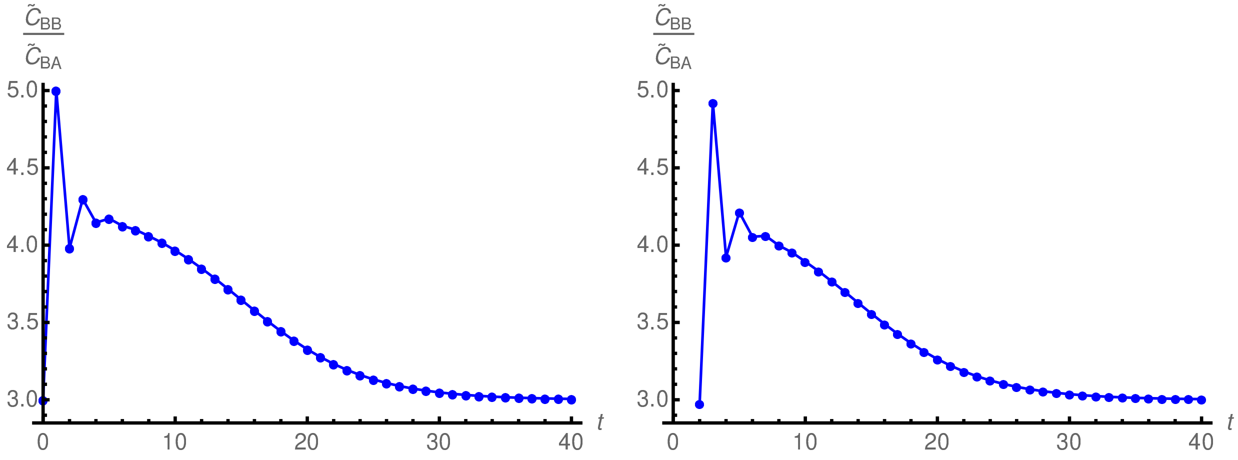


(a) (b)

Figure 5. Ratio $\widetilde{C}_{\mathrm{BB}}/\widetilde{C}_{\mathrm{BA}}$ in the five state model system. a): locally equilibrated initial distribution in Markov state B, $\mathbf{y}^T(0) = (0, \frac{1}{2}, \frac{1}{2})$; b): locally non-equilibrated initial distribution in Markov state B, $\mathbf{y}^T(0) = (0, 1, 0)$. Because the initial population of $y_2(0) = 0$, the points only start after $y_2$ has gained some population (here: after two MC steps).

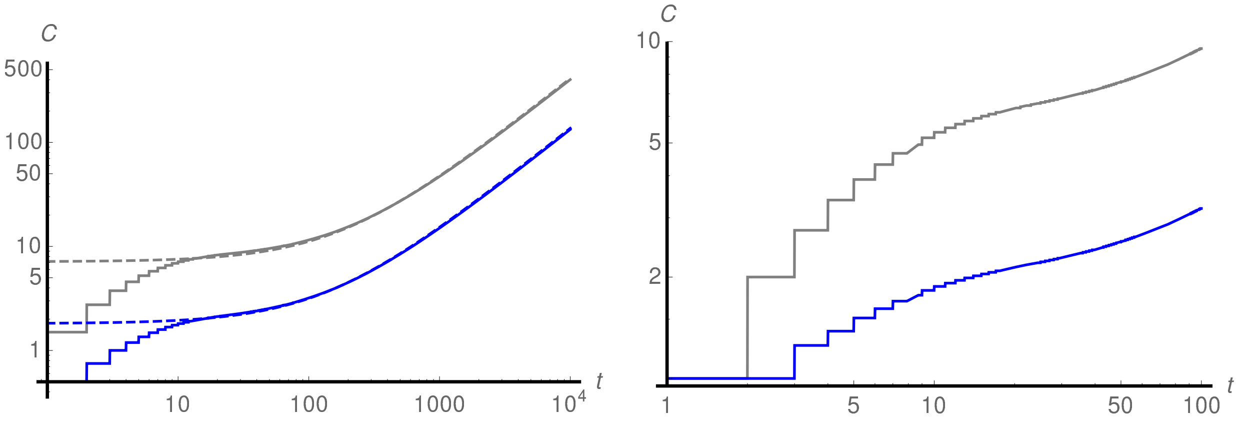


(a) (b)

Figure 6. Total numbers of transitions $C_{\mathrm{BB}}$ (grey) and $C_{\mathrm{BA}}$ (blue) in the five state model system. a): locally equilibrated initial distribution in Markov state B, $\mathbf{y}^T(0) = (0, \frac{1}{2}, \frac{1}{2})$, b): locally non-equilibrated initial distribution in Markov state B, $\mathbf{y}^T(0) = (0, 1, 0)$.

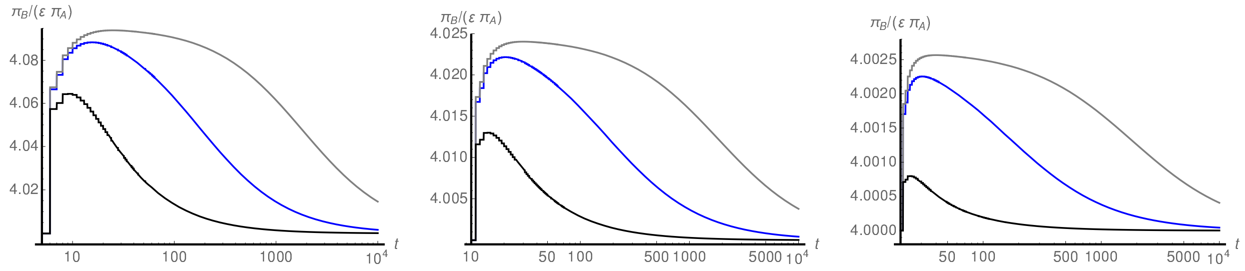


(a) (b) (c)

Figure 7. Evolution of the ratio $\frac{\pi_\mathrm{B}}{\varepsilon\pi_\mathrm{A}}$ with the number of MC steps for an initial probability vector of $\mathbf{y}^T(0) = (0, \frac{1}{2}, \frac{1}{2})$ and lag times $\tau = 5$ MC steps (a), $\tau = 10$ MC steps (b) and $\tau = 20$ MC steps (c), respectively.

## Solution for a system with two Markov states and random connections between microstates

As mentioned in the main text, we consider a system with two Markov states with $n_\mathrm{A}$ and $n_\mathrm{B}$ microstates, each microstate having connections to $k$ randomly chosen other microstates. For this system we calculate the bias $\hat{\pi} = \frac{\pi_\mathrm{B}}{\pi_\mathrm{A}\,\varepsilon}$ in the limit of low temperatures as a function of $n_\mathrm{A}, n_\mathrm{B}$ and $k$, with $n_\mathrm{A} + n_\mathrm{B} = 200$. For this purpose, we average over 50 independent randomly chosen connectivities. As suggested in the main text, we plot the result as a function of $n_\mathrm{B}/(kn_\mathrm{A})$; see Fig. **??**. One can clearly see that for small values of $n_\mathrm{B}$ one indeed observes a superposition for the data with connectivities 6, 8, 12. Furthermore, going to larger values of $n_\mathrm{B}$ the resulting bias depends on the connectivity: the higher the connectivity, the smaller the bias. Finally, around $n_\mathrm{B}/(kn_\mathrm{A}) \approx 0.5$ one observes the crossover between the behavior at large and small number of microstates in the upper Markov state. Intuitively, one might have expected a value larger than unity because only then there have to exist microstates in the upper Markov states which are not connected to the lower Markov state. Due to the random nature of the connectivity, even at a value of 0.5 there exist a larger number of microstates in the upper Markov state which are not connected to the lower Markov state. This seems to be sufficient to produce the maximum bias for the given connectivity.

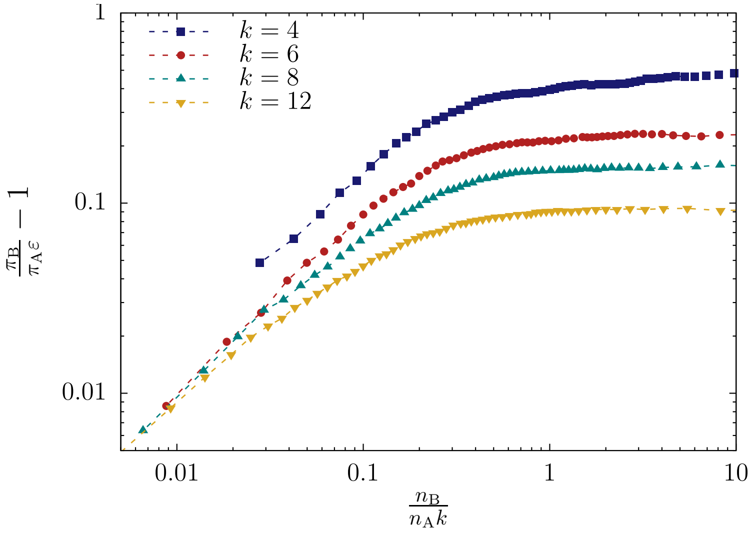


Figure 8. MSM estimation bias $\frac{\pi_B}{\pi_A \varepsilon} - 1$ in a system with $n_A + n_B = 200$ microstates that are grouped into two Markov states A and B as a function of $n_A, n_B$ and $k$. Each microstates has $k$ randomly chosen connections to other microstates.

## Accounting for absent connections in the MSM estimation process

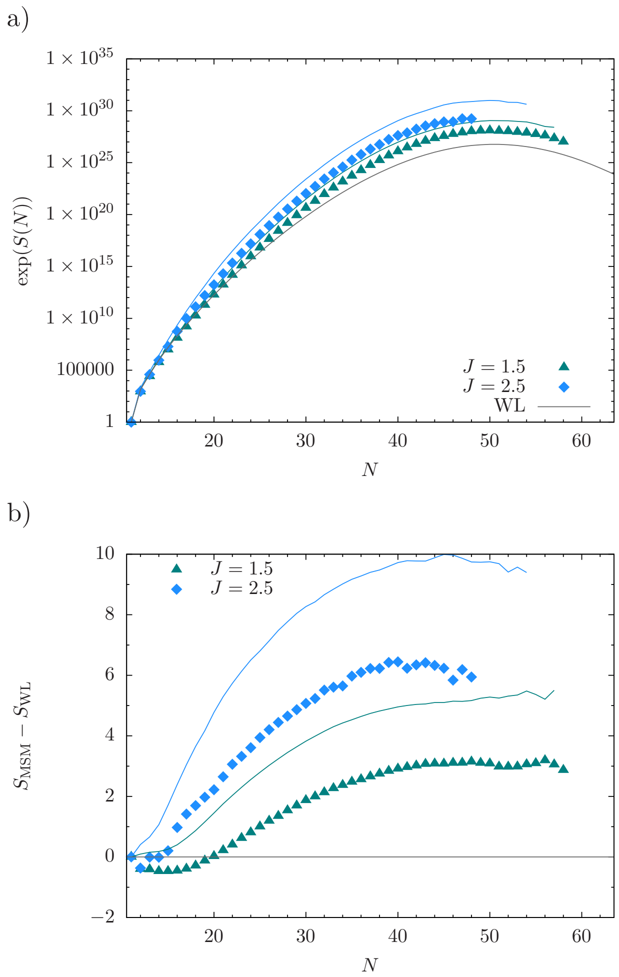


Figure 9. Density of states $g(N) = \exp(S(N))$ (a) and the difference in the entropies $S_{\mathrm{MSM}} - S_{\mathrm{WL}}$ (b) as a function of the order parameter $N$ in a system of size $m^2 = 10^2$. The colored lines correspond to the results from MSM that have been obtained without using the algorithm, the grey line represents the density of states from the WL algorithm and the colored symbols correspond to the new results from MSM with the new algorithm.
